# Supplementary material for: Affinity LCFCN: Learning to Segment Fish with Weak Supervision
Source: arXiv:2011.03149 source file (2020-11-06)
Supplement: Supplementary file 1 [file additional_material.tex]

\documentclass[10pt,twocolumn,letterpaper]{article}

\usepackage{wacv}
\usepackage{times}
\usepackage{epsfig}
\usepackage{graphicx}
\usepackage{amsmath}
\usepackage{amssymb}
\usepackage{caption}
\usepackage{subcaption}
\usepackage{pgfplots}
\usepackage{comment}
\usepackage{array, makecell} %
\usepackage[numbers]{natbib}
\bibliographystyle{plainnat}
\setlength{\bibsep}{0.0pt}

% Include other packages here, before hyperref.

% If you comment hyperref and then uncomment it, you should delete
% egpaper.aux before re-running latex.  (Or just hit 'q' on the first latex
% run, let it finish, and you should be clear).
\usepackage[pagebackref=true,breaklinks=true,letterpaper=true,colorlinks,bookmarks=false]{hyperref}

% \cvprfinalcopy % *** Uncomment this line for the final submission

 % Enter the WACV Paper ID here

%(2)
%\wacvfinalcopy % *** Uncomment this line for the final submission

%(3)
\ifwacvfinal
 % *** Enter the assigned starting page number (instead of 9876)
\fi
% Optional math commands from https://github.com/goodfeli/dlbook_notation.
\input{math_commands.tex}

\begin{document}

%%%%%%%%% TITLE
\title{Approximate Online Bilevel Optimization for Learning Data Augmentation\\Additional material}

%%%%%%%%%%%%%%%%%%%%%%
% AUTHORS
%%%%%%%%%%%%%%%%%%%%%%
\author{Saypraseuth Mounsaveng\\
\'Ecole de Technologie Sup\'erieure\\
Montr\'eal, Canada\\
{\tt\small saypraseuth.mounsaveng.1@etsmtl.net}
\and
David Vazquez\\
Element AI\\
Montreal, Canada\\
{\tt\small dvazquez@elementai.com}
\and
Ismail Ben Ayed\\
\'Ecole de Technologie Sup\'erieure\\
Montr\'eal, Canada\\
{\tt\small ismail.benayed@etsmtl.ca}
\and
Marco Pedersoli\\
\'Ecole de Technologie Sup\'erieure\\
Montr\'eal, Canada\\
{\tt\small marco.pedersoli@etsmtl.ca}
}
\maketitle
%\thispagestyle{empty}

%%%%%%%%%%%%%%%%%%%%%
% Additional material
\section{Implementation details}

We use PyTorch to implement our experiments, and Kornia library for the color transformations.

\subsection{Model architecture}
Table~\ref{tab:C} shows  the BadGAN classifier architecture. Table~\ref{tab:A} shows the augmenter network for affine and color transformations. Finally,  Table~\ref{tab:A_mask} shows the details of the augmenter network for mask transformations.

\begin{table}[ht]
\centering
\footnotesize
%\resizebox{\columnwidth}{!}{%
\begin{tabular}{c}
\textbf{Classifier C}\\
\hline
Input 32x32 Image\\
\hline
3x3 conv. 96 LReLU(0.2)\\
3x3 conv. 96 LReLU(0.2)\\
3x3 conv. 96 LReLU(0.2), 0.5 dropout\\
3x3 conv. 192 LReLU(0.2)\\
3x3 conv. 192 LReLU(0.2)\\
3x3 conv. 192 LReLU(0.2), 0.5 dropout\\
3x3 conv. 192 LReLU(0.2)\\
3x3 conv. 192 LReLU(0.2)\\
3x3 conv. 192 LReLU(0.2)\\
MLP 10 unit, sigmoid\\
10-class Softmax\\
\end{tabular}
%}
\caption{\textbf{BadGAN classifier network}.}
\label{tab:C}
\end{table}

\begin{table}[ht]
\centering
\footnotesize
%\resizebox{\columnwidth}{!}{%
\begin{tabular}{c|c|c}
\multicolumn{3}{c}{\textbf{Augmenter A}}\\
\hline
\textit{Small} & \textit{Medium} & \textit{Large}\\
\hline
Input $n^*$ dim. & Input 100 dim. & Input 100 dim.\\
\hline
MLP $n$ units & MLP 64 unit & MLP 512 unit\\
relu, 0.2 dropout & relu, 0.2 dropout & relu, 0.2 dropout\\
MLP 10 x $n$ units & MLP 32 unit & MLP 1024 unit\\
relu, 0.2 dropout & relu, 0.2 dropout & relu, 0.2 dropout\\
- & - & MLP 1024 unit\\
- & - & relu, 0.2 dropout\\
- & - & MLP 512 unit\\
- & - & relu, 0.2 dropout\\
\hline
\multicolumn{3}{c}{MLP $n$ units, tanh}\\
\end{tabular}
%}
\caption{\textbf{Augmenter network for affine and color transformations}. For \textit{Small}, $n$ is the number of parameters to learn (6 for affine, 4 for color and 10 when combining both).}
\label{tab:A}
\end{table}

\begin{table}[ht]
\centering
\footnotesize
%\resizebox{\columnwidth}{!}{%
\begin{tabular}{c}
\textbf{Augmenter A}\\
\hline
Input 100 dim.\\
\hline
8x8 deconv. 8\\
2x2 deconv. 16\\
2x2 deconv. 32\\
1x1 deconv. 3\\
\end{tabular}
%}
\caption{\textbf{Augmenter network for mask transformations}.}
\label{tab:A_mask}
\end{table}

\subsection{Affine transformation parameters}
In our experiments, we use affine transformations. The augmenter network learns a 2x3 matrix containing the parameters of the affine transformations.

\subsection{Color transformation parameters}
We use the following color transformations in our experiments: i) Hue in range [-0.5:0.5]; ii) Saturation in range [0:1]; iii) Contrast in range [-1:1] iv) Brightness in range [0:1]. In all cases the zero value corresponds to the identity transformation.

\section{Additional experiments}
We investigate the influence of augmenter regularization on the model performance.
Figure~\ref{fig:regularization} shows the model performance for different weight decay values. This indicates that the model is not sensitive to regularization.

\begin{figure}[h]
    \centering
    \resizebox{\columnwidth}{!}{%
    \begin{tikzpicture}
        \begin{axis}[
            legend cell align={left},
            xtick=data,
            width=\columnwidth,
            height=.4\columnwidth,
            % major x tick style = transparent,
            symbolic x coords={0.001, 0.01, 0.1},
            bar width=10pt,
            enlarge x limits=0.25,
            ybar,
            ymajorgrids,
            ymin=90,
            ylabel= Accuracy (\%),
            xlabel= Weight decay value,
            % legend image code/.code={%
            %     \draw[#1, draw=none] (0cm,-0.1cm) rectangle (0.3cm,0.1cm);
            % },  
            % legend style={
            %     legend style={row sep=-3pt},
            %     draw=none,
            %     font=\small,
            %     legend pos=outer north east,
            % }
            legend style={at={(0.5,01.50)},
    anchor=north,legend columns=3},
        ]
        \addplot[fill=blue] coordinates {(0.1, 94.84) (0.01, 94.86) (0.001, 94.39)};
        \addplot[fill=green] coordinates {(0.1, 92.48) (0.01, 91.73) (0.001, 91.43)};
        \addplot[fill=orange] coordinates {(0.1, 94.81) (0.01, 94.93) (0.001, 94.43)};        
        \legend{affine, color, full }
        \end{axis}
    \end{tikzpicture}
    }
        \caption{\textbf{Augmenter regularization.} Accuracy for different weight decay values for the augmenter (affine, color and the combination of both) with ResNet18 on CIFAR10.}
    \label{fig:regularization}
    \vspace{-4mm}
\end{figure}

% \subsection{Comparison with SotA}

% To assess the performance of our model on bigger networks, we evaluated our model using a Wide ResNet 28-10 classifier. On Table \ref{tab:comparison_sota_wrn}, we can that our model is amazing.

% \begin{table}[h!]
% \centering
% \resizebox{\columnwidth}{!}{%
% \begin{tabular}{l|c|c|c}
%     \textbf{Classifier} & \textbf{CIFAR10} & \textbf{CIFAR100}\\
%     \hline
%     Baseline (WRN 28-10)      & 94.83 & 68.99 \\
%     Predefined (WRN 28-10) & xx & xx \\
%     \hline
%     AutoAugment (WRN 28-10)   & 97.40 & 82.90 \\
%     Fast AA (WRN 28-10)       & 97.30 & 82.70 \\
%     PBA (WRN 28-10)           & 97.40 & 83.30 \\
%     RandAugment (WRN 28-10)   & 97.30 & 97.30 \\\hline   
%     Our model (WRN 28-10)     & \textbf{xx} & \textbf{xx} \\
% \end{tabular}%
% }
% \caption{\textbf{Comparison with SotA on Wide ResNet 28-10}. Our model based on affine, color, and mask transformations outperforms most of the previous methods for automatic and manual data augmentation.
% }
% \label{tab:comparison_sota_wrn}
% \end{table}

\end{document}
